# Supplementary material for: Sample and Communication-Efficient Decentralized Actor-Critic Algorithms with Finite-Time Analysis
Source: arXiv:2109.03699 source file (2022-02-03)
Supplement: Supplementary file 1 [file appendix.tex]

\clearpage
\onecolumn
\appendix
